# Supplementary material for: From Attention to Activation: Unravelling the Enigmas of Large Language Models
Source: arXiv:2410.17174 source file (2024-10-22)
Supplement: Supplementary file 1 [file 04-sm1.tex]

\section{Method: First Token Domination}\label{sec:meth-first-token}
In this section we shall eliminate certain plausible causes of the two anomalies in transformer models.
We shall primarily consider GPT2 as a representative transformer model, due to its simplicity,
but also consider Llama models to narrow down the potential causes of the anomalies.
In all our experiments, unless stated otherwise, we use a GPT2 model with $\sim$130M parameters
trained on the \texttt{en} split of the C4 dataset.
The various changes we make to the model are described throughout the paper
as we eliminate potential causes of the anomalies. 

\subsection{Eliminating Certain Causes}\label{ssec:elim-first-token}
Given that GPT2 models and Llama models both exhibit the first token dominance in attention maps,
we only consider the parts of the transformer architecture that are common to both models
as potential causes of this anomaly.
GPT2 and Llama architectures differ in the following aspects:
% reduce spacing before itemize
\begin{itemize}[noitemsep,topsep=0pt]
    \setlength\itemsep{0em} % reduce itemize spacing
    \item Llama models use Rotary Positional Encodings (RoPE)~\citep{su2024roformer}, while GPT2 models uses learnt absolute positional encodings~\citep{vaswani2017attention}.
    \item Llama models use a \texttt{<bos>} token to denote the beginning of a sequence, while GPT2 models do not.
    \item Llama models use SiLU~\citep{elfwing2018sigmoid} activations in the feedforward layers, while GPT2 models use GeLU activations~\citep{hendrycks2016gaussian}.
    \item Llama models use RMSNorm~\citep{zhang2019root} as the normalisation layer, while GPT2 models use LayerNorm~\citep{ba2016layer}.
\end{itemize}
Although, Llama and GPT2 use different kinds of positional encodings, they both do use some kind of positional encodings.
Therefore it is plausible that the positional encodings privilege the first token in a way
that leads to the first token dominance in attention maps.
The remaining differences between the two models listed above do not affect the first token differently
compared to other tokens~\ie~the normalisation layer and the activation function are applied identically to all token positions.
Therefore, we train a GPT2 model \emph{without any positional encodings} and observe the attention maps,
comparing them to another GPT2 model trained with learnt absolute positional encodings, all other parameters and hyperparameters being the same.

We find the GPT2 model without (with) positional encodings
exhibits first token dominance in 33\% (20\%) of the (query, head) pairs and
allocates 17\% (10\%) of all attention to the first key
(as in \cref{ssec:pd-first-token}, evaluation is performed on the validation set of the \texttt{en} split of the C4 dataset).
Despite a small reduction in first token dominance, the anomaly persists in the model without positional encodings,
therefore we conclude that the positional encodings are not the cause of the first token dominance in attention maps.

\subsection{Removing First Token Dominance of Attention Maps}\label{ssec:first-token-sol}
In the previous section we eliminated positional encodings as a potential cause of the first token dominance in attention maps.
Some other aspects of Transformer models were dismissed as potential causes of the anomaly due to
their action being invariant to the token position.
We blame a combination of two aspects of Transformer models which lead to first token dominance:
(1) the causal masking of self-attention in language models, and
(2) softmax normalisation of the attention scores.
The causal masking of self-attention (\ie~the masking which prevents tokens from attending to future tokens during training)
is the strictest form of privilege the first token receives in the model.

Consider the self-attention mechanism on the initial token positions in a transformer model with causal masking.
The first query token can only attend to its own key and due to the softmax normalisation, it receives an attention score of 1.
Similarly, the second query token can only attend to its own key and the first key,
and due to the softmax normalisation, the attention scores must sum to 1.
There are many works which demonstrate a given attention head specialises to a particular concept or
group of concepts~\citep{voita2019analyzing,bansal2023rethinking}.
Despite this, when a given input sequence is not relevant to an attention heads' specialisation,
it must still allocate attention summing to 1 (due to the softmax normalisation) and
the causal masking of self-attention privileges the first (key) token above all other tokens as
it is the only key token to which \emph{all} queries can attend (due to the causal masking).
This explains why any particular token position dominates the attention maps and specifically,
why the \emph{first} token dominates the attention maps, rather than any other token position.

Previous works have suggested solutions to the first token dominance in attention maps, such as
adding registers (extra learnt tokens forming part of the input sequence)~\citep{darcet2024vision} or clipping the softmax
function and adding gating to the attention scores~\citep{bondarenko2023removing}.

We propose a much simpler solution to the first token dominance anomaly by simply
modifying the softmax normalisation of the attention scores.

Consider the canoncial softmax function on a logit vector $\mathbf{x} \in \real^L$,
where $L$ is the sequence length:
\begin{align}
    \text{softmax}(x_i) &= \frac{\exp(x_i)}{\sum_{j=1}^{L} \exp(x_j)} \\
    \sum_{i=1}^{L} \text{softmax}(x_i) &= 1
\end{align}
we see that even if logit scores for (query, key) pairs are all small, the softmax normalisation
enforces that the attention scores sum to 1 leading to the first token dominance anomaly.
We propose a simple modification to the softmax function:
\begin{align}
    \text{softmax-1}(x_i) &= \frac{\exp(x_i)}{1 + \sum_{j=1}^{L} \exp(x_j)} \\
    \sum_{i=1}^{L} \text{softmax-1}(x_i) &< 1
\end{align}
where we add a constant 1 to the denominator of the softmax function.
This modification removes the strict normalisation of the attention scores to 1 and allows the model to
allocate attention scores as it sees fit \ie~low logit scores across all (query, key) pairs will result in
low attention scores across all (query, key) pairs.
In the limit of one or more logit scores being very large, the softmax-1 function will approach the canonical softmax function.
Note that we only modify the softmax function in the self-attention mechanism and not in the final language modeling head which predicts the next token
across the model vocabulary.

Looking at this modification from the ``registers'' perspective, the constant 1 in the denominator
of the softmax-1 function can be thought of as a register (key) token which always has logit score 0 with
respect to all queries.

We train a GPT2 model with the softmax-1 function and observe the attention maps,
comparing them to another GPT2 model trained with the canonical softmax function, all other parameters and hyperparameters being the same
(\ie~both models have learnt absolute positional encodings).
We find that the GPT2 model with the softmax-1 (canonical softmax) function exhibits first token dominance in 2\% (53\%) of the (query, head) pairs and
allocates 4\% (46\%) of all allocated attention to the first key.
Note that because of the softmax-1 function, the attention scores are not enforced to sum to 1 and
therefore the \emph{sum of all attention scores across all (query, head) pairs is not the same as that in the model with canonical softmax function}.
We find that the softmax-1 model allocates $\sim$45\% of the attention compared to the canonical softmax model.

Figure xyz shows the average attention maps of our GPT2 models trained with: (1) canonical softmax and learnt position encodings (standard model);
(2) canonical softmax and no positional encodings; and (3) softmax-1 and learnt position encodings.

Importantly, we find the training of the GPT2 model with the softmax-1 function is stable and almost identical to the training of the standard GPT2 model in
terms of convergence and perplexity on the validation set of the C4 dataset
(please see the appendix for comparative training curves between the models mentioned in this section and for details on the training procedure we use).

\subsection{Discussion}\label{ssec:disc-first-token}
We have shown that the first token dominance in attention maps is a result of the causal masking of self-attention,
which privileges the first token position above all other tokens,
combined with the softmax normalisation of the attention scores forcing the total attention allocated in a given (query, head) pair to sum to 1.
Our proposed a simple modification to the softmax function, which removes the strict normalisation of the attention scores to 1,
results in a model which does not demonstrate first token dominance in attention maps.
The softmax-1 function has been mentioned previously in a short blogpost which discusses softmax-1 as the solution to
the \emph{outlier activations in the residual stream} not the first token dominance in attention maps~\citep{miller2023attention}.
Figure xyz shows the mean absolute value of the activations in the hidden states of a GPT2 model trained with the canonical softmax function (with and without positional encodings)
and the softmax-1 function (with positional encodings).
We find that the only significant change in the outlier activations is that the extreme outliers observed in the first token position
of the hidden states of the GPT2 model trained with the canonical softmax function (with or without positional encodings) are no longer present in the GPT2 model trained with the softmax-1 function,
which is intuitive as softmax-1 removes the privilege of the first token position in the attention maps over all other token positions.
However, the general outlier activations in specific feature channels across all token positions remain in the GPT2 model trained with the softmax-1 function.
Therefore, we conclude that the first token dominance in attention maps and the outlier activations in the residual stream are not related and
a separate solution is required to address the latter anomaly.

% Considering a single head of self-attention given hidden states $\mathbf{X} \in \real^{L \times D}$,
% where $L$ is the sequence length and $D$ is the hidden dimension, self-attention in a single head is given by
% \begin{align}
%     \text{Attention}(\mathbf{X}; \mathbf{W}_Q, \mathbf{W}_K, \mathbf{W}_V) = \text{softmax}\left(\frac{\mathbf{Q}\mathbf{K}^T}{\sqrt{D}}\right)\mathbf{V},
% \end{align}
