# Supplementary material for: From Attention to Activation: Unravelling the Enigmas of Large Language Models
Source: arXiv:2410.17174 source file (2024-10-22)
Supplement: Supplementary file 2 [file 00-appendix_plan.tex]

\section{Plan}\label{sec:plan}

\begin{itemize}
    \item Appendix structure
    \item Maths behind kurtosis
    \item All the stuff about orthogonal transformations and inf-2norm ratio
    \item Loss Curves - ours, ablation
    \item training details
    \item examples of pretrained models with first token domination (todo)
\end{itemize}
Split up the per layer plots
